# Supplementary material for: First-Principles-Based Strain and Temperature Dependent Ferroic Phase Diagram of SrMnO$_3$
Source: arXiv:1807.04777 ancillary file (2018-07-12)
Supplement: Supplementary file 1 [file suppl.pdf]

# Supplementary Material: First-Principles-Based Strain and Temperature Dependent Ferroic Phase Diagram of $SrMnO_3$

Alexander Edström and Claude Ederer
*Materials Theory, ETH Zürich, Wolfgang-Pauli-Strasse 27, 8093 Zürich, Switzerland*

# I. HEISENBERG EXCHANGE INTERACTIONS AND MAGNON SPECTRA

## A. Deviation from Ideal Heisenberg Behavior

For an ideal Heisenberg magnet, the computed exchange interactions for a pair of atomic magnetic moments should be independent of the configuration of magnetic moments on the other atoms than those in that pair. In real materials there will, however, be some degree of dependence on the magnetic reference state considered. Fig. 1 shows the first nearest neighbor exchange interactions as functions of strain, calculated with respect to different magnetic structures, including G, C ($\mathbf{q} = (1, 0, a/c)\pi/a$), and A-type ($\mathbf{q} = (0, 0, 1)\pi/c$) AFM, as well as the FM state. Additionally, cubic $CaMnO_3$ nearest neighbor interactions, calculated with respect to G-type AFM and FM states, are shown for comparison. It is clear that the exchange interactions of $SrMnO_3$ do depend on the magnetic reference state, although the qualitative trend as a function of strain is unchanged. This indicates a form of non-Heisenberg behaviour. However, since there is merely some amount of quantitative vertical shift in the exchange interactions as functions of strain for different magnetic reference states, it is not expected to qualitatively affect the results of our work. It can also be noted that such an effect is also present in $CaMnO_3$.

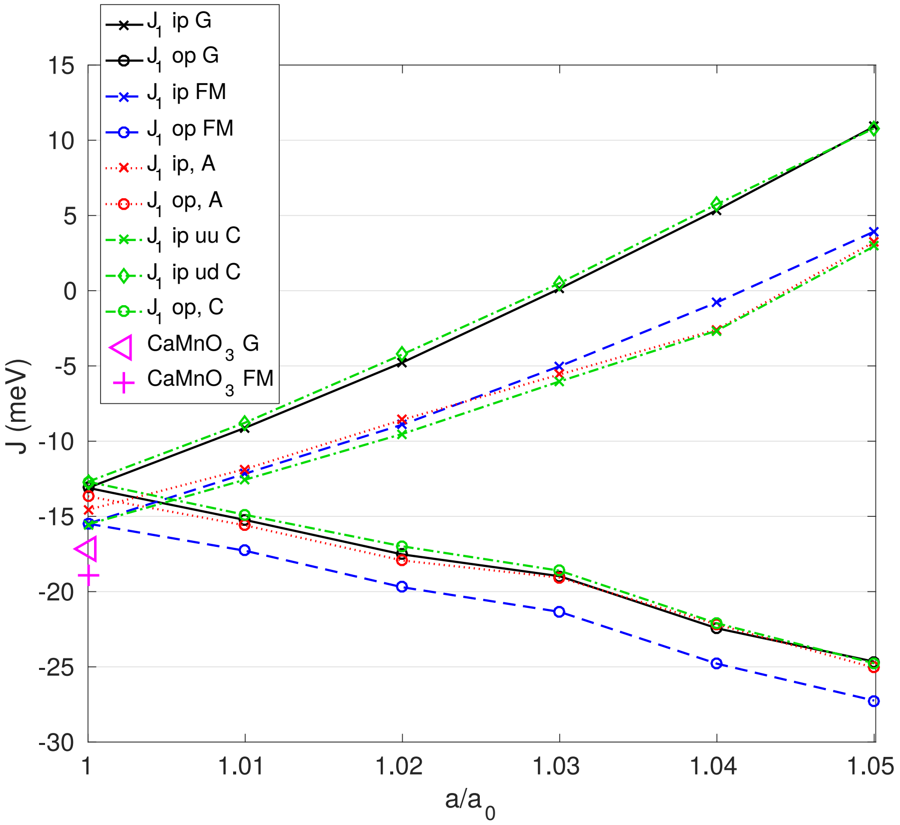


Figure 1: Heisenberg exchange parameters as function of strain, calculated with respect to different reference magnetic structures. The exchange interactions of cubic $CaMnO_3$, with respect to FM and G-type AFM magnetic structures are also shown.

In the cubic structure ($a/a_0 = 1$), the two different nearest neighbor interactions, $J_1^{\text{ip}}$ and $J_1^{\text{op}}$, should be equal by symmetry. This is the case for the calculations with respect to FM or G-type AFM magnetic structures, as these magnetic states retain the cubic symmetry. However, for A and C-type AFM, this is no longer the case. Furthermore, in the case of C-AFM, $J_1^{\text{ip}}$ is further split into two different values depending on whether one considers the bond which is parallel (uu) or anti-parallel (ud) in the reference state, although in the cubic structure $J_1^{\text{ip,ud}} = J_1^{\text{op}}$.

As strain is introduced, one can observe that $J_1^{\text{ip}}$ and $J_1^{\text{op}}$ are each split into two groups, depending on whether the given pair of magnetic moments is parallel or anti-parallel in the reference structure considered. For example, for $J_1^{\text{ip}}$, the value calculated for a G-AFM structure is very similar to the antiparallel in-plane interaction for C-type AFM. The dependence on computed exchange interactions in transition metal oxide compounds on magnetic reference states

and exchange-correlation functionals was discussed recently and it was suggested that spin-independent functionals yield a more Heisenberg-like behaviour [1].

### B. Effect of Hubbard U on Calculated Exchange Parameters

Fig. 2 shows the first and second nearest neighbour exchange interactions as functions of $U$, for a fixed cubic structure with G-type AFM and $a_0 = 3.79$ Å. The magnitudes of the exchange interactions decrease with increasing $U$. This is in agreement with expectations, since in a superexchange model the exchange interaction is inversely proportional to the Hubbard $U$ [2], even though the exchange interactions in Fig. 2 do not follow a simple $U^{-1}$ behaviour. The mean field Curie temperature is also shown in Fig. 2 and it decreases with increasing $U$, since the magnitudes of the exchange interactions decrease. In the main text, it is found that Monte Carlo simulations of the Heisenberg Hamiltonian with exchange interactions evaluated with $U = 3$ eV underestimate the experimental critical temperature by 33% (175 K from Monte Carlo simulations compared to 233 K from experiments [3]). According to the data in Fig. 2, $U = 1.5$ eV would lead to a 33% increase in $T_{\mathrm{C}}$ compared to the value obtained with $U = 3$ eV. However, it is also seen from Fig. 2 that an increase in the magnitude of the exchange interactions in the range 10-20% is obtained by calculating them with respect to a ferromagnetic reference state. Thus, it is not clear how much of the discrepancy in $T_{\mathrm{C}}$ is due to choosing a suitable value for $U$, and how much is due to non-Heisenberg behaviour.

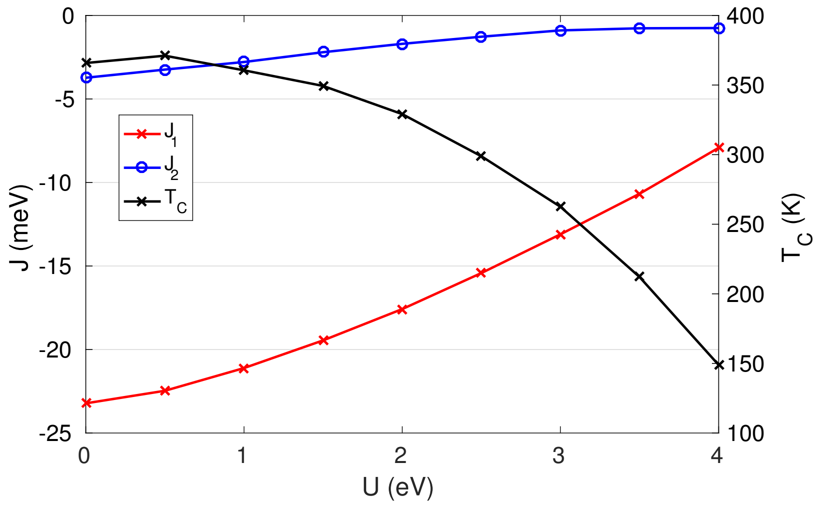


Figure 2: Heisenberg exchange interactions, for cubic G-type AFM $SrMnO_3$, as well as the mean field critical temperature, as functions of the Hubbard $U$.

### C. Adiabatic Magnon Spectra

Fig. 3 contains the adiabatic magnon spectra for various strains $\eta$. These are computed according to [4, 5]

$$E(\mathbf{q}) = \hbar\omega(\mathbf{q}) = \frac{2\mu_{\mathrm{B}}}{M}\left[J(0) - J(\mathbf{q})\right], \tag{1}$$

where $M$ is the Mn magnetic moment, $\mu_{\mathrm{B}}$ is the Bohr magneton and

$$J(\mathbf{q}) = \sum_i J_{0i} \mathrm{e}^{\mathrm{i}\mathbf{q}\cdot\mathbf{R}_i}, \tag{2}$$

with $J_{0i}$ denoting the exchange interaction between atom 0 and atom $i$, and $\mathbf{R}_i$ being the position of atom $i$ relative to atom 0. $E(\mathbf{q})$ describes the energy of a magnetic configuration labeled by $\mathbf{q}$ relative to the FM state. That $E(\mathbf{q})$ is mainly negative indicates that the ferromagnetic state is unstable, i.e. other spin configurations are lower in energy. At small strains, the minimum in $E(\mathbf{q})$ occurs at the $\mathbf{q} = (1, 1, a/c)\frac{\pi}{a}$ $\mathbf{q}$-vector (the units of the $\mathbf{q}$-vectors are $\pi/a$ for the first two components and $\pi/c$ for the last component), which corresponds to G-type AFM. At 3% strain the

minimum is at $(0, 1, 1)$ (equivalent to $(1, 0, 1)$), i.e. C-type AFM, while at larger strains the minimum is at $(0, 0, 1)$ (A-type AFM).

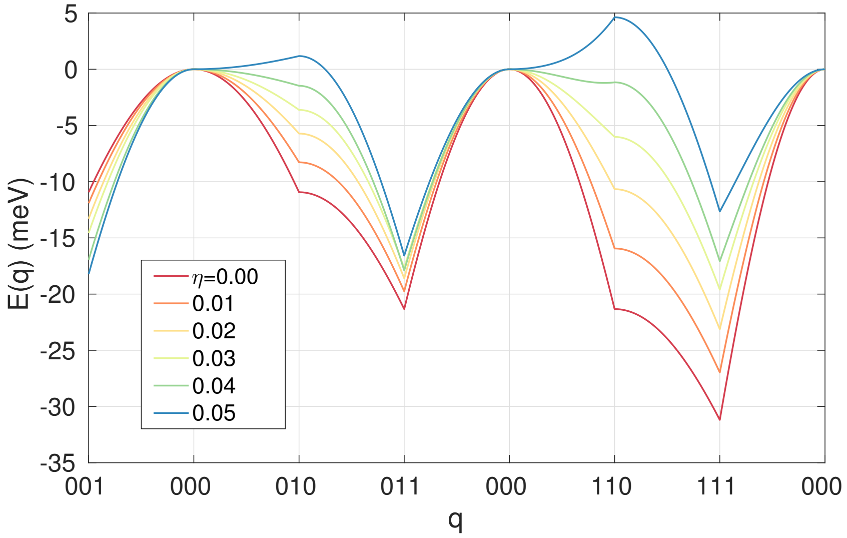


Figure 3: Adiabatic magnon spectra for $SrMnO_3$ with various strains.

## II. COMPUTING THE PARAMETERS FOR THE FE EFFECTIVE HAMILTONIAN

### A. Soft Phonon Mode Displacement Pattern

Table I contains the (imaginary) frequencies and (normalized) displacement vectors for the unstable polar phonon mode at various strains. $O_x$ denotes the oxygen atom located at $\pm a\hat{x}/2$ away from the Mn atom, and correspondingly for $y$ and $z$. For negative strain ($a/a_0 < 1$) the atomic displacements are in the $z$-direction, while for positive strain ($a/a_0 > 1$), the atomic displacements are in the $x$-direction (equivalently they could be chosen in the $y$-direction, corresponding to a degenerate phonon mode, which would exchange $\xi_{O_x}$ and $\xi_{O_y}$). For a phonon mode in the cubic perovskite structure, only two different oxygen displacements would appear, corresponding to one oxygen atom positioned parallel ($O_\parallel$) or two perpendicular ($O_\perp$) to the displacement direction, respectively. For negative strain, this is also the case for the displacements in Table I. However, for positive strain, which is the main focus of this work, there is an additional symmetry breaking, as the out-of-plane direction is different from the in-plane direction perpendicular to the displacement direction. In the cubic structure, the five three-fold degenerate phonon modes can be divided into four modes with $\Gamma_{15}$ symmetry and one with $\Gamma_{21}$ symmetry [6]. The latter displaces the two $O_\perp$ in opposite directions. The tetragonal symmetry breaking in the strained structure allows the $\Gamma_{21}$-mode to mix with the other modes and this leads to the reduced symmetry of the displacements for positive strain in Table I, i.e. different displacements for all three oxygen atoms. The lines marked with a "$*$" in Table I show the displacement patterns that result if one projects out the contribution from the $\Gamma_{21}$-mode, thus re-instating the cubic symmetry.

Since the soft mode displacement changes with strain, one could argue for considering this as a strain dependent variable and computing also the remaining parameters of the effective Hamiltonian as functions of strain. However, this is in practice cumbersome and, furthermore, is in conflict with the main idea of the effective Hamiltonian approach. Since the change in the soft mode displacement vector with strain additionally does not appear too substantial, we will make a choice of fixing it to that found for 3% strain. As the effective Hamiltonian is derived considering small deviations from a cubic perovskite structure, it appears desirable to use a soft mode displacement vector consistent with the cubic symmetry. Thus, we also choose to use the symmetry-modified version of the displacement vector, in the row of Table I for $a/a_0 = 1.03$ marked with a "$*$". It is interesting to note the similarity between this displacement pattern with that for $a/a_0 = 0.95$, when exchanging $O_x$ and $O_z$, indicating that it is feasible to use the same soft mode displacement vector and parametrisation also for negative strain.

For comparison, the line marked by a † also shows the displacements, away from the high symmetry positions of the atoms, in the relaxed structure with 3% strain, after projecting out an arbitrary contribution from the accoustic phonon mode. The resulting displacements are similar to the displacement pattern obtained, for the same strain,

Table I: Soft mode frequencies and corresponding displacement vectors (with displacements in the $x$ or $z$-directions, depending on if the strain is positive ot negative), for various strains. The two lines marked by a "$*$" show the symmetry modified displacement patterns, according to the discussion in the text. The line marked with a † shows the normalized displacements of the atoms in the relaxed structure with 3% strain.

| $a/a_0$ | f (Thz) | $\xi_{\mathrm{Sr}}$ | $\xi_{\mathrm{Mn}}$ | $\xi_{\mathrm{O}_x}$ | $\xi_{\mathrm{O}_y}$ | $\xi_{\mathrm{O}_z}$ |
|---|---|---|---|---|---|---|
| 0.95 | 3.84i | 0.0289 | 0.4049 | −0.4460 | −0.4460 | −0.6614 |
| 0.96 | 1.52i | 0.0334 | 0.3971 | −0.4715 | −0.4715 | −0.6298 |
| 1.03 | 4.21i | 0.0389 | 0.3869 | −0.6596 | −0.3505 | −0.5393 |
| 1.04 | 6.27i | 0.0266 | 0.3986 | −0.7157 | −0.3123 | −0.4803 |
| 1.03* | 4.21i | 0.0392 | 0.3904 | −0.6655 | −0.4489 | −0.4489 |
| 1.04* | 6.27i | 0.0268 | 0.4015 | −0.7208 | −0.3991 | −0.3991 |
| 1.03† | - | 0.0767 | 0.3618 | −0.6281 | −0.3470 | −0.5902 |

from phonon calculations. This is a reassuring indication that the infinitesimal displacement pattern obtained from phonon calculations actually can provide a good description of the finite sized FE displacements.

### B. Elastic Constants

With the soft mode displacement pattern established, most other parameters can be determined by performing total energy calculations for various structural distortions. The elastic coefficients, $B_{11}$, $B_{12}$ and $B_{44}$ are obtained as in Ref [7]. That is, by computing the total energy for structural distortions caused by strain tensors

$$\bar{\bar{\epsilon}} = \begin{pmatrix} 0 & 0 & 0 \\ 0 & 0 & 0 \\ 0 & 0 & \eta \end{pmatrix}, \quad \bar{\bar{\epsilon}} = \begin{pmatrix} \eta & 0 & 0 \\ 0 & \eta & 0 \\ 0 & 0 & \eta \end{pmatrix}, \quad \bar{\bar{\epsilon}} = \frac{1}{2}\begin{pmatrix} 0 & \eta & \eta \\ \eta & 0 & \eta \\ \eta & \eta & 0 \end{pmatrix} \tag{3}$$

and fitting these energies to

$$E(\eta) = E_0 + \frac{1}{2}B_{11}\eta^2, \tag{4}$$

$$E(\eta) = E_0 + \frac{3}{2}(B_{11} + B_{12})\eta^2, \tag{5}$$

and

$$E(\eta) = E_0 + \frac{3}{2}B_{44}\eta^2, \tag{6}$$

respectively. The calculated points and fitted curves are shown in Fig. 4.

### C. Self Energy Parameter

The self-energy parameters, $\kappa$, $\alpha$, $\gamma$ and $k_i$, occur in an energy expression of the form

$$\begin{aligned} E(\mathbf{u}) =& \kappa u^2 + \alpha u^4 + \gamma\left(u_y^2 u_z^2 + u_y^2 u_z^2 + u_y^2 u_z^2\right) + k_1 u^6 + k_2\left[u_x^4(u_y^2 + u_z^2) + u_y^4(u_x^2 + u_z^2) + u_z^4(u_x^2 + u_y^2)\right] \\ &+ k_3 u_x^2 u_y^2 u_z^2 + k_4 u^8 \end{aligned} \tag{7}$$

for a homogeneous polarisation ($\mathbf{u}_i = \mathbf{u}_j = \mathbf{u}$, $\forall i, j$). Note that the quadratic parameter $\kappa$ contains contributions from the local mode self-energy ($\kappa_2$), as well as inter-site couplings. The self-energy parameters are evaluated by computing the total energy for polarizations along crystallographic [100], [110] and [111]-directions, i.e., $\mathbf{u} = (u, 0, 0)$, $\mathbf{u} = \frac{u}{\sqrt{2}}(1, 1, 0)$ and $\mathbf{u} = \frac{u}{\sqrt{3}}(1, 1, 1)$. Calculations are thus performed to obtain the total energy as function of atomic displacements $\mathbf{u}\xi_A$, where $A$ denotes an atomic species and $\xi_A$ the numbers contained in Table I. The calculated

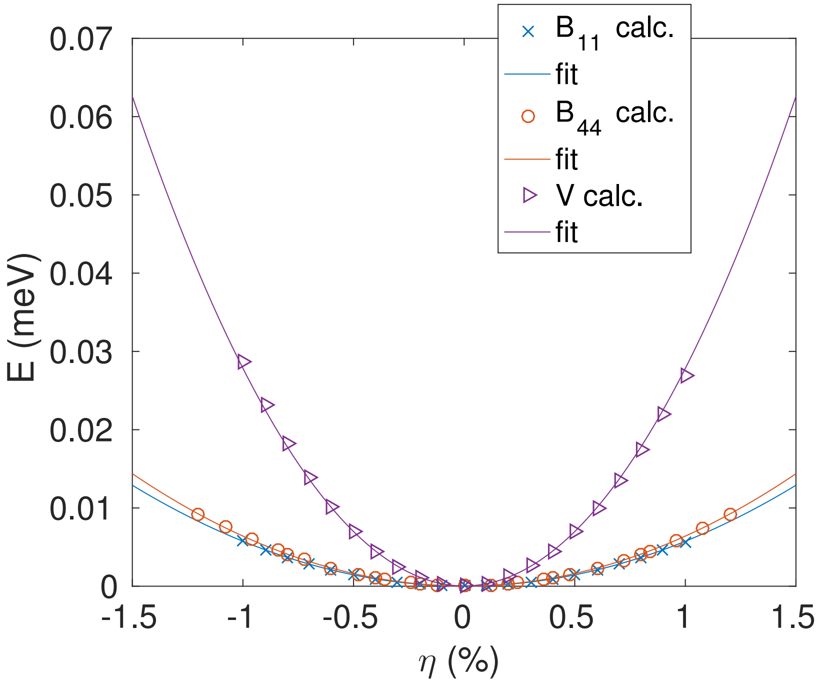


Figure 4: Energy as function of various strains, used to evaluate the elastic constants.

energies as function of soft mode displacements, together with a fitting to the energy expression in Eq. 7, are shown in Fig. 5. This is similar to how these parameters were determined in Ref. [7], with the difference that all the data points, for different polarization directions, are simultaneously fitted in Fig. 5, while in Ref. [7] the fitting is first done for the [100]-direction, which fixes $\kappa$, $\alpha$, $k_1$ and $k_4$. The remaining curves are then only used for determining the remaining parameters. The single fitting performed here leads to one consistent set of parameters, where the data computed for the three different polarization directions are treated on equal footing.

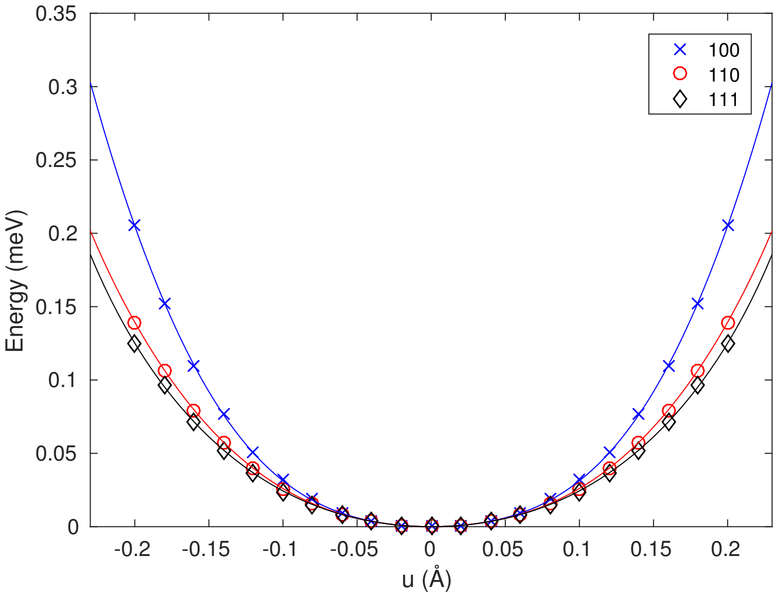


Figure 5: Energy as function of soft mode amplitude for homogenous polarisations along different crystal directions, computed via DFT and fitted curves.

### D. Strain-Mode Coupling

The strain-mode coupling parameters $B_{1xx}$, $B_{1yy}$, and $B_{4yz}$, are also computed similarly as in Ref. [7], somewhat differently from how it is done in Refs. [8,9]. In Ref. [9], the parameters are found by calculating the forces on atoms as function of strain with a frozen in soft mode displacement. Here, and in Ref. [7], various soft mode displacements are frozen in, and for each of these the energy-minimizing strain ($\eta_{\mathrm{eq}}$) is computed. The parameters are then calculated by fitting of the strain-mode curves that are obtained.

For a homogeneous polarization, the strain-mode interaction energy is

$$E_{\mathrm{int}}(\mathbf{u}, \bar{\bar{\epsilon}}) = \frac{1}{2} \sum_{i\alpha\beta} B_{i\alpha\beta} \eta_i u_\alpha u_\beta. \tag{8}$$

Note that the strain tensor

$$\bar{\bar{\epsilon}} = \begin{pmatrix} \epsilon_{xx} & \epsilon_{xy} & \epsilon_{xz} \\ \epsilon_{yx} & \epsilon_{yy} & \epsilon_{yz} \\ \epsilon_{zx} & \epsilon_{zy} & \epsilon_{zz} \end{pmatrix} = \begin{pmatrix} \eta_1 & \eta_6/2 & \eta_5/2 \\ \eta_6/2 & \eta_2 & \eta_4/2 \\ \eta_5/2 & \eta_4/2 & \eta_3 \end{pmatrix} \equiv (\eta_1, \eta_2, \eta_3, \eta_4, \eta_5, \eta_6) \tag{9}$$

is described in Voigt notation. The energy minimizing strain $\eta_{\mathrm{eq}}$ is computed for the three different cases

$$\mathbf{u} = u\hat{x} \quad \text{and} \quad \bar{\bar{\epsilon}} = \eta(1, 0, 0, 0, 0, 0), \tag{10}$$

$$\mathbf{u} = u\hat{x} \quad \text{and} \quad \bar{\bar{\epsilon}} = \eta(0, 0, 1, 0, 0, 0), \tag{11}$$

and

$$\mathbf{u} = \frac{u}{\sqrt{2}}(\hat{x} + \hat{y}) \quad \text{and} \quad \bar{\bar{\epsilon}} = \eta(0, 0, 0, 0, 0, 1). \tag{12}$$

According to the effective Hamiltonian, $\eta_{\mathrm{eq}}$ should increase proportionally to $u^2$ in each of these cases. The strain-mode coupling parameters are then obtained from the fittings and conversions

$$\eta_{\mathrm{eq}} = a_{1xx} u^2, \quad B_{1xx} = -2B_{11} a_{1xx}, \tag{13}$$

$$\eta_{\mathrm{eq}} = a_{1yy} u^2, \quad B_{1yy} = -2B_{11} a_{1yy} \tag{14}$$

and

$$\eta_{\mathrm{eq}} = a_{4yz} u^2, \quad B_{4yz} = -2B_{44} a_{4yz}, \tag{15}$$

for the structural distortions in Eqs. 10-12, respectively. The resulting calculated and fitted $\eta_{\mathrm{eq}}(u)$ curves are shown in Fig. 6.

In Fig. 6(a)-(b), $\eta_{\mathrm{eq}}$ is indeed proportional to $u^2$ and it is unproblematic to extract $B_{1xx}$ and $B_{1yy}$. However, in Fig. 6(c), such a relation only appears to hold for small $u$, while for larger $u$ higher order effects are clearly important. If one does the quadratic fitting only in the range where it produces a relatively good fit, e.g. the points marked with red crosses but excludes the points at larger $u$, marked by blue circles, one obtains a value of $B_{4yz} = -26.26$ eV/Å$^{-2}$. Such a value will, however, clearly overestimate the coupling of the soft FE mode to shear strain for the larger $u$ values which are relevant for the larger strains considered in this work. It was found that this overestimate of the shear strain led to domain formations at low temperatures, that do not appear to be consistent with DFT calculations. Thus, the energy as function of $u$ from the effective Hamiltonian was computed for a $32 \times 32 \times 32$-system, with homogeneous polarisation, as well as for a system with a 90° domain wall perpendicular to the (100)-direction separating (1,1,0) and (1,-1,0) polarised domains. Within each domain, the polarisation is homogenous and each dipole has equal magnitude. The energy difference for the system with a domain minus the energy for a homogeneously polarised system is shown in Fig. 7. Attempts at supercell DFT calculations did not indicate any tendencies to favor domain formation, which is considered as a motivation to choose $B_{4yz}$ small enough that domains are not favored over the homogeneously polarised state. According to Fig. 7, choosing $B_{4yz} = -10$ eV/Å$^{-2}$ allows the homogeneously polarised state to be favored over the whole range of $u$ considered. Thus, this is chosen as the value of $B_{4yz}$. Note that in a homogeneously polarised state, no shear strain appears, which makes the precise value of $B_{4yz}$ less important in many cases of interest.

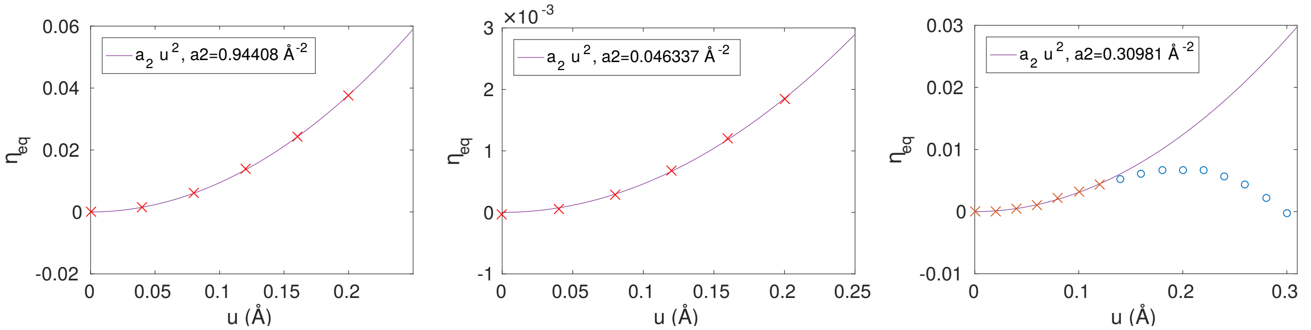


(a) $B_{1xx}$ (b) $B_{1yy}$ (c) $B_{4yz}$

Figure 6: $\eta_{\mathrm{eq}}(u)$ for different structural distortions, calculated from DFT (red crosses and blue circles), and fitted quadratic curves. The data points marked with blue circles in (c) have been exluded from the curve fitting.

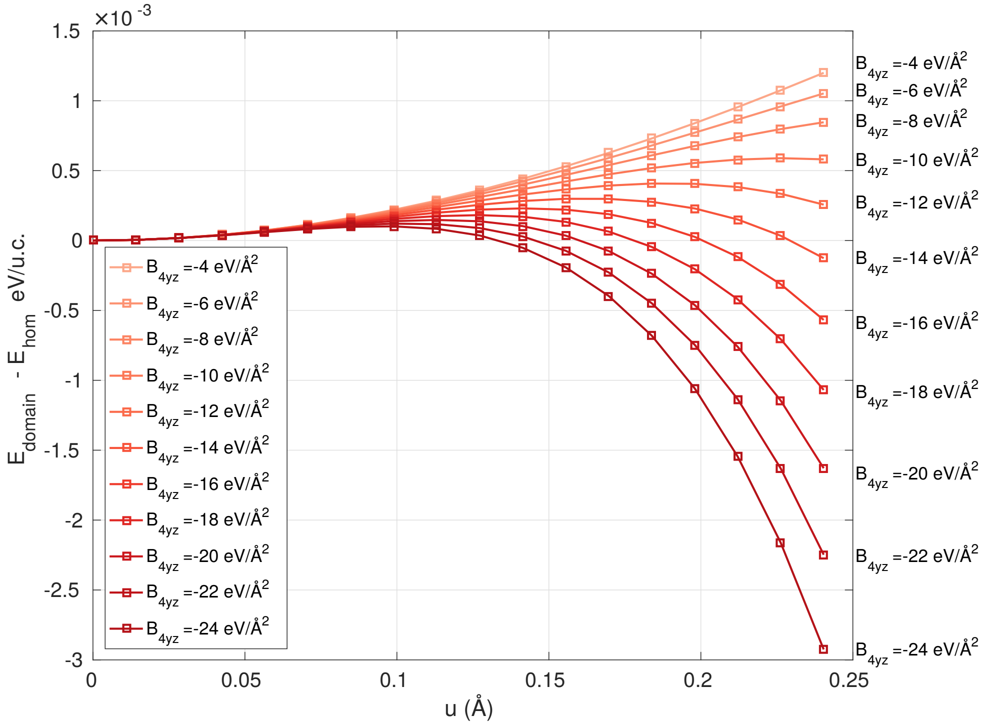


Figure 7: Energy as function of $u$ for a system with domains minus that of a system without domain, from the effective Hamiltonian, calculated using FERAM.

### E. Short-Range Interaction Parameters

The short-range interaction parameters $j_k$ occur in an energy expression of the form

$$E_{\mathrm{short}}(\{\mathbf{u}\}) = \frac{1}{2}\sum_{i\neq j}\sum_{\alpha\beta} J_{ij,\alpha\beta} u_{i\alpha} u_{j\beta}, \tag{16}$$

where $i, j$ denote sites and $\alpha, \beta$ denote cartesian components. The parameters $J_{ij,\alpha\beta}$, for the first three nearest neighbours, which are considered in this work, can be expressed in terms of the parameters $j_k$ according to [8]

$$\begin{aligned} \text{First neighbor:} \quad & J_{ij,\alpha\beta} = \left[j_1 + (j_2 - j_1)\left|\hat{R}_{ij,\alpha}\right|\right]\delta_{\alpha\beta} \\ \text{Second neighbor:} \quad & J_{ij,\alpha\beta} = \left[j_4 + \sqrt{2}(j_3 - j_4)\left|\hat{R}_{ij,\alpha}\right|\right]\delta_{\alpha\beta} + 2j_5\hat{R}_{ij,\alpha}\hat{R}_{ij,\beta}\left(1-\delta_{\alpha\beta}\right) \\ \text{Third neighbor:} \quad & J_{ij,\alpha\beta} = j_6\delta_{\alpha\beta} + 3j_7\hat{R}_{ij,\alpha}\hat{R}_{ij,\beta}\left(1-\delta_{\alpha\beta}\right), \end{aligned} \tag{17}$$

where $\hat{R}_{ij}$ is the unit vector from site $i$ to site $j$. As discussed in the main text, $j_5$ and $j_7$ are set to zero. Fig. 1 in Ref. [8] contains a geometric description of the different $j_k$. These parameters are, furthermore, essentially determined in the same way as in Ref. [8], i.e. by computing the energy when freezing in displacement patterns, of the local soft mode, according to wavevectors $\Gamma = (0,0,0)$, $X = (1,0,0)\frac{\pi}{a}$, $M = (1,1,0)\frac{\pi}{a}$ and $R = (1,1,a/c)\frac{\pi}{a}$ in the Brillouin zone. In practice this is done by computing the total energy for supercells containing $2\times2\times2$ perovskite unit cells, with dipolar arrengements according to the Fig. 2(a)-(f) in Ref. [8] and a small $u$ (here $u = 0.01$ Å). Finally, the $j_k$ are determined by solving the linear system of equations described by Eq. 15(a)-(f) in Ref. [7].

As discussed in the main text, it was necessary to introduce strain dependent $j_k$ in this work, in order for the effective Hamiltonian to agree with the results of the DFT calculations. The symmetry breaking caused by tetragonal strain would imply that a larger number of short range interactions are needed. However, considering tensile strain and assuming that the polarisation is always in the $xy$-plane, it is sufficient to consider only the parameters of the Hamiltonian based on the cubic structure. Thus, the frozen phonon total energy calculations are performed for polarisations in the plane and one set of calculations is done for each strain considered. Furthermore, the dielectric constant enters Eq. 15 in Ref. [7] and this is also considered strain dependent in these equations. Finally, when the system is strained, a contribution $\frac{u^2}{2}\left[\eta_1(B_{1xx}+B_{1yy})+\eta_3 B_{1yy})\right]$ appears in the total energy, whereby this is subtracted from the total energy before solving the equations for $j_k$.

### F. Energy landscape of the effective Hamiltonian

The situation explored in the current work, where an biaxial tensile strain is applied, effectively corresponds to fixing the strain tensor to $\eta = (\eta_1, \eta_1, \eta_3, 0, 0, 0)$, where $\eta_1$ is fixed, while $\eta_3$ is allowed to relax. This typically results in a polarisation in the (110)-direction, i.e. $\mathbf{u} = (1,1,0)u/\sqrt{2}$. Assuming a homogenous polarisation the energy becomes

$$\begin{aligned} E(\eta,u) =& \frac{B_{11}}{2}\left(2\eta_1^2+\eta_3^2\right) + B_{12}\left(\eta_1^2 + 2\eta_1\eta_3\right) + \left[\kappa_2 + J - \frac{2}{3}\frac{\pi\hbar c\tilde{\alpha}Z^*}{\epsilon_\infty a^3} + \frac{1}{2}\left(\eta_1(B_{1xx}+B_{1yy}) + \eta_3 B_{1yy}\right)\right]u^2 \\ &+ (\alpha+\gamma/4)\,u^4 + (k_1+k_2/4)\,u^6 + k_4 u^8, \end{aligned} \tag{18}$$

where $J = 2j_1 + j_2 + 4j_3 + 2j_4 + 4j_6$, $\hbar$ is the reduced Planck's constant, $c$ the speed of light in vacuum and $\tilde{\alpha}$ is the fine structure constant. Minimising the energy with respect to $\eta_3$, i.e. imposing $\frac{\partial E}{\partial \eta_3} = 0$, yields

$$\eta_3 = -\frac{1}{B_{11}}\left(2B_{12}\eta_1 + \frac{1}{2}B_{1yy}u^2\right). \tag{19}$$

Inserting Eq. 19 into Eq. 18 results in

$$\begin{aligned} E(\eta_1,u) =& \eta_1^2\left(B_{11}+B_{12}-\frac{B_{12}^2}{B_{11}}\right) + \left[\kappa_2 + J - \frac{2}{3}\frac{\pi\hbar c\tilde{\alpha}Z^*}{\epsilon_\infty a^3} + \frac{1}{2}\eta_1\left(B_{1xx} + B_{1yy}(1-2\frac{B_{12}}{B_{11}})\right)\right]u^2 \\ &+ \left(\alpha+\gamma/4 - \frac{1}{8}\frac{B_{1yy}^2}{B_{11}}\right)u^4 + (k_1+k_2/4)\,u^6 + k_4u^8 \end{aligned} \tag{20}$$

$$= A_0 + A_1u^2 + A_2u^4 + A_3u^6 + A_4u^8. \tag{21}$$

In this work, $\kappa_2$, $J$ and $\epsilon_\infty$ are also considered as functions of $\eta_1$.

Fig. 8 shows the energy as function of $u$ for different $\eta_1$ from Eq. 20. Energy minima at $u \neq 0$ develops for $\eta_1 = 2.5\%$ and higher. The $u$ yielding the minimum energies in Fig. 8 and the corresponding $\eta_3$ from Eq. 19 are the quantities plotted in Fig. 6 in the main text.

[1] S. Keshavarz, J. Schött, A. J. Millis, and Y. O. Kvashnin, Phys. Rev. B **97**, 184404 (2018).

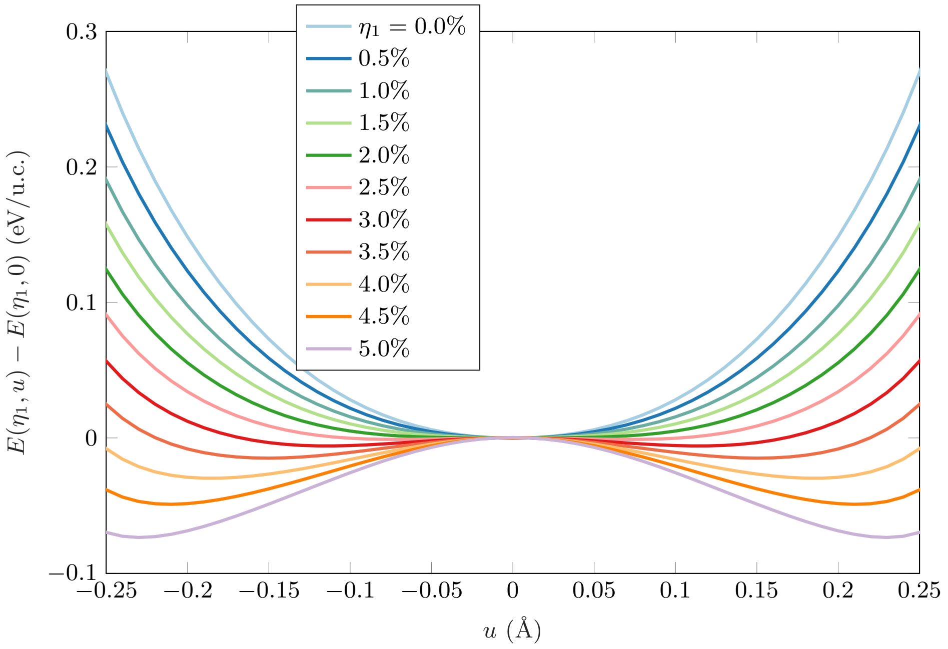


Figure 8: Energy as function of $u$ according to the effective Hamiltonian, with homogeneous polarisation along [110], for various strains $\eta_1$.

[2] P. W. Anderson, in *Solid State Physics*, Vol. 14, edited by F. Seitz and D. Turnbull (Academic Press, 1963) pp. 99 – 214.
[3] L. Maurel, N. Marcano, T. Prokscha, E. Langenberg, J. Blasco, R. Guzmán, A. Suter, C. Magén, L. Morellón, M. R. Ibarra, J. A. Pardo, and P. A. Algarabel, Phys. Rev. B **92**, 024419 (2015).
[4] S. V. Halilov, H. Eschrig, A. Y. Perlov, and P. M. Oppeneer, Phys. Rev. B **58**, 293 (1998).
[5] M. Pajda, J. Kudrnovský, I. Turek, V. Drchal, and P. Bruno, Phys. Rev. B **64**, 174402 (2001).
[6] M. S. Dresselhaus, G. Dresselhaus, and A. Jorio, *Group Theory* (Springer, Heidelberg, 2008).
[7] T. Nishimatsu, M. Iwamoto, Y. Kawazoe, and U. V. Waghmare, Phys. Rev. B **82**, 134106 (2010).
[8] W. Zhong, D. Vanderbilt, and K. M. Rabe, Phys. Rev. B **52**, 6301 (1995).
[9] R. D. King-Smith and D. Vanderbilt, Phys. Rev. B **49**, 5828 (1994).
